# Supplementary material for: Kiki or Bouba? Sound Symbolism in Vision-and-Language Models
Source: arXiv:2310.16781 source file (2024-04-02)
Supplement: Supplementary file 1 [file appendix.tex]

\input{supp-gen}
\input{supp-phonetics}
\input{supp-models}
\input{supp-qual}
\input{supp-lex}
\input{supp-unimodal}
